# Supplementary material for: Chiral transport and electronic correlations in surface states of HfNiSn single crystals
Source: arXiv:1805.06337 source file (2018-05-16)
Supplement: Supplementary file 1 [file supplement.pdf]

# Supplemental material for the manuscript *"Chiral transport and electronic correlations in surface states of HfNiSn single crystals"*

L. Steinke[1], J. J. Kistner-Morris[2], T. F. Lovorn[3], H. He[1], A. D. Hillier[4], P. Miao[1], S. Zellman[1], M. Klemm[1], O. Gonzalez[1], M. Green[1], A. H. MacDonald[3] and M. C. Aronson[1]
[1] *Department of Physics and Astronomy, Texas A & M University, College Station, TX 77845, USA*
[2] *Department of Physics and Astronomy, Stony Brook University, Stony Brook, New York, USA*
[3] *Department of Physics and Astronomy, University of Texas, Austin, TX , USA*
[4] *ISIS Facility, STFC Rutherford Appleton Laboratory, Chilton, Oxfordshire, OX11 0QX, UK*
(Dated: January 31, 2018)

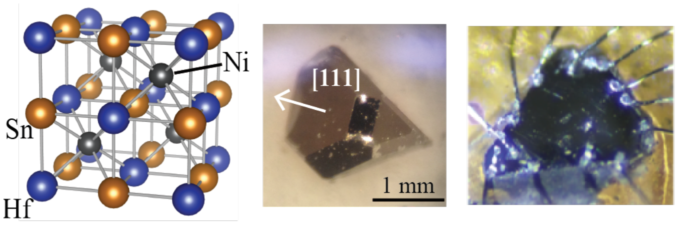


FIG. 1. **a**: Crystal structure of HfNiSn. **b**: photograph of a flux-grown HfNiSn single crystal. **c**: transport sample fabricated by sanding a single crystal down to a coplanar platelet parallel to the main (111) facet.

| $T$ (K) | a (Å) | GoF | R | wR |
|---|---|---|---|---|
| 298 | 6.0721(2) | 1.122 | 0.0189 | 0.0413 |
| 100 | 6.06300(10) | 1.200 | 0.0178 | 0.0447 |

TABLE I. X-ray structure parameters for a HfNiSn single crystal. No structural transitions are observed between 300 K and 100 K.

## I. SAMPLES AND EXPERIMENTAL SETUP

HfNiSn single crystals were grown from Sn self-flux, forming well-faceted polyhedra with typically one large [111]-facet. The face-centered cubic C1b half-Heusler structure (Fig. 1a) with space group F-43m and a lattice constant of 6.07 Å was verified by X-ray structure analysis at 300 K and 100 K (Table I), and wavelength-dispersive spectroscopy (WDS) confirms a near-stoichiometric composition and high purity of the HfNiSn single crystals.

The magnetic properties of HfNiSn single crystals were measured in a Quantum Design Magnetic Properties Measurement System (MPMS), and magnetotransport measurements were performed in a Quantum Design Physical Properties Measurement System (PPMS). Electrical transport samples were polished to obtain a coplanar platelet in the shape of the main [111]-facet (Fig. 1), with typical facet diameters of 1-2 mm and a sample thickness between 0.1 - 0.2 mm. Contacts were placed along the edge of the sample by direct ultrasonic bonding of 33 $\mu$m thick aluminum wires to the HfNiSn crystal.

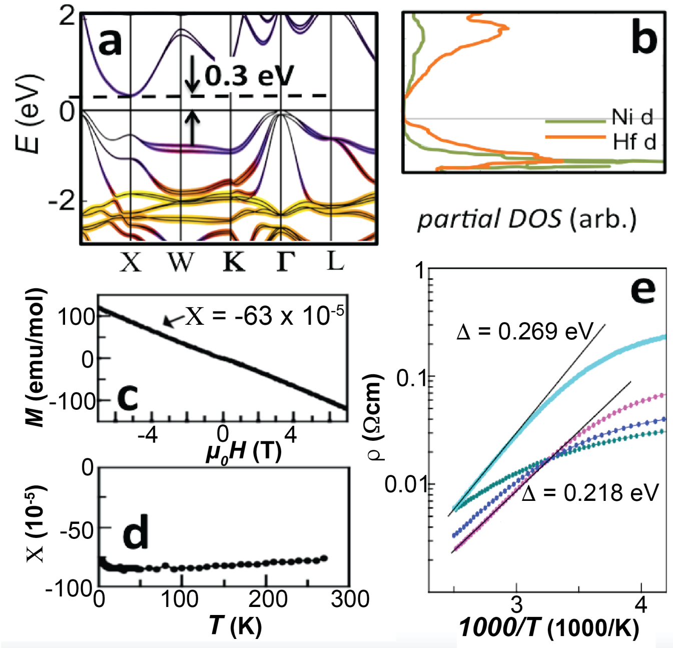


FIG. 2. **HfNiSn is a bulk diamagnetic insulator.** **a**: DFT calculation of the band structure, with an overlaid color map indicating the partial density of states for Hf and Ni d-orbitals plotted in panel **b**. **c**: $M(H)$ of a 3.4 mg HfNiSn single crystal at $T = 1.8$ K. **d**: $T$-dependent magnetization in a field of 10 Oe. **e**: Arrhenius plot of electrical resistivity $\rho(T)$ for different samples, with exponential fits indicating a band gap close to the calculated value in **a**.

## II. BULK DIAMAGNETIC INSULATOR

DFT calculations using the structure parameters from single crystal X-ray measurements predict HfNiSn to be an insulator with no band inversion and a small indirect band gap of 0.3 eV (Fig. 2a), which agrees well with the value obtained from the thermally activated temperature $T$-dependent resistivity $\rho$ (panel e) above 200 K, and is consistent with the temperature dependence of the Hall effect (Fig. 3). At low temperatures, the $T$-dependence of the resistance (Fig. 4) measured in the local 4-point configuration sketched in the inset is ambiguous between two-dimensional (2D) or three-dimensional variable-range hopping characterized by dif-

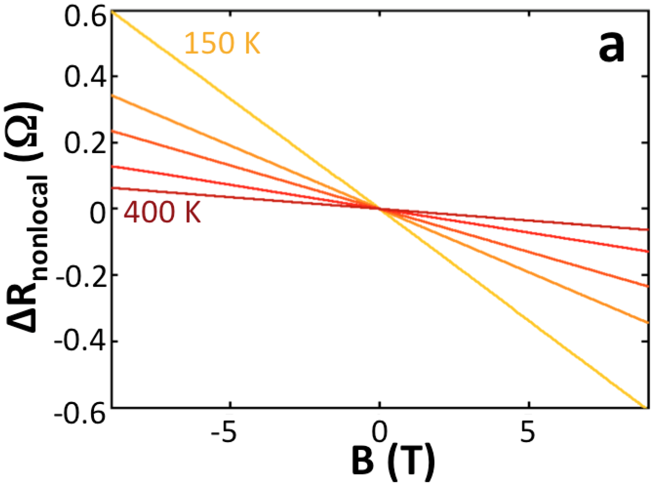


FIG. 3. Hall effect measured in a HfNiSn single crystal sample with the magnetic field perpendicular to the main (111) facet. The increasing slope with decreasing temperature is consistent with the freeze-out of activated carriers between 400 K and 150 K.

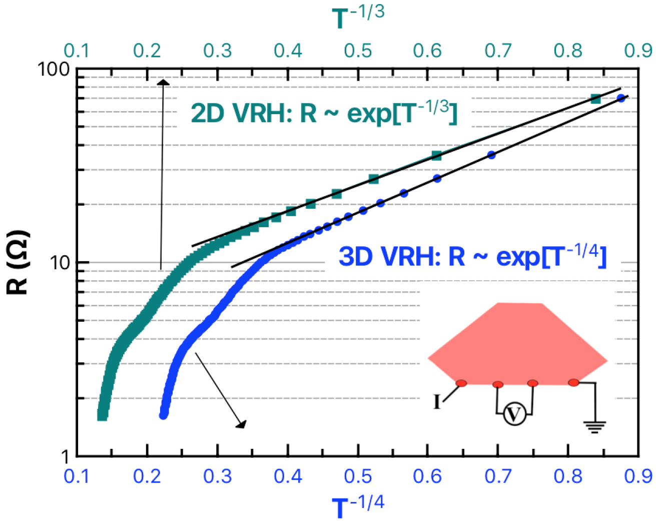


FIG. 4. Temperature dependence of the local transport component, measured in the 4-point configuration sketched in the inset.

ferent power law dependencies: charges could either be traveling through localized states in the bulk of the HfNiSn single crystal or in 2D surface states. The overlaid color map in Fig. 2a indicates the partial density of states of Hf and Ni d-orbital states, plotted separately in panel b. Both Hf and Ni d-orbital states are removed from the Fermi surface, and the broad energy distribution indicates strong hybridization, which is expected to suppress magnetism from local magnetic moments. In agreement with these DFT results, measurements of the magnetic properties (Fig. 2c and d) show that HfNiSn is diamagnetic with a weakly temperature-dependent susceptibility, ruling out a strong magnetic character. This result is consistent with muon spin rotation ($\mu$ SR) measurements [1] shown in Fig. 5. The time-dependent depolarization of the muon beam (decreasing asymmetry) could either be caused by static nuclear moments only, or by a combination of static nuclear moments and weak magnetic fluctuations of electron spins. The absence of periodic oscillations rules out a strong internal magnetic field from the ordering of electron spins.

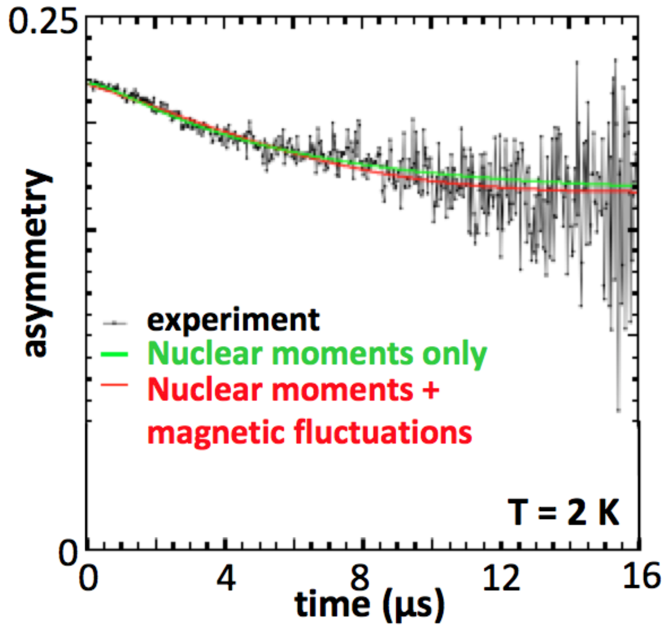


FIG. 5. $\mu$ SR data measured on a 400 mg batch of HfNiSn single crystals. The red line is a fit to $A_s G_z(t) = A_0 \exp(-\Lambda t) G_{GKT}(t) + A_{bg}$, where $A_0$ is the initial asymmetry, $A_s$ and $A_{bg}$ correspond to the sample contribution and background, with $A_0 + A_{bg} = A_s$. $\Lambda$ is the relaxation rate due to dynamic spin-lattice-relaxation. $G_{GKT}(t)$ is the static Gaussian Kubo-Toyabe relaxation function related to the nuclear spin distribution. The green line is a fit to $A_s G_z(t) = A_0 G_{DGKT}(t) + A_{bg}$, where $G_{DGKT}(t)$is the dynamic Gaussian Kubo-Toyabe relaxation function which also relates to the nuclear spin distribution.

---

[1] The $\mu$ SR measurements were performed at the high-field muon instrument, HiFi, at the ISIS facility. The software package Mantid was used for data analysis. http://aip.scitation.org/doi/full/10.1063/1.4972827
